# Supplementary material for: Trustworthy Machine Learning under Distribution Shifts
Source: arXiv:2512.23524 source file (2025-12-29)
Supplement: Supplementary file 1 [file appendix.tex]

\section{Appendix A}

Something
